# Supplementary material for: Closed form expression for the 5-point Veneziano amplitude in terms of 4-point amplitudes
Source: arXiv:2111.02423 ancillary file (2021-11-03)
Supplement: Supplementary file 1 [file A5_Expressions.pdf]

# Closed-form expressions for the 5-point open string tachyon amplitudes: definitions

Bogdan Stoica  
Northwestern University  
bstoica@gmail.com

---

## Gelfand - Graev objects

(\*These objects are not needed for any of the new 5-point amplitude results below. They are included for convenience.\*)

Gelfand-Graev gamma function for multiplicative character  $|\cdot|(^S)$ .

$$\Gamma_{GG}[S_] := 2^{(1-S)} \pi^{-S} \cos[(\pi * S) / 2] \Gamma[S];$$

Total 4 - point Veneziano amplitude (summed over all orderings of momenta)

$$A_{4GG}[S_, T_] := (\Gamma_{GG}[S + 1] * \Gamma_{GG}[T + 1]) / \Gamma_{GG}[S + T + 2];$$

---

## The 5 - point amplitude in terms of 4 - point amplitudes

4 - point Veneziano amplitude for one ordering of momenta

$$A_4[S_, T_] := (\Gamma[1 + S] \Gamma[1 + T]) / \Gamma[2 + S + T];$$

Full (120-permutation symmetric) 5 - point Veneziano amplitude in terms of 4-point amplitudes and 6F5 hypergeometric functions.

$$A_{5InTermsof6F5}[S2_, T2_, S3_, T3_, M23_] := \\ 4 A_4[M23 + S2, T2] * A_4[S3, T3] \text{HypergeometricPFQ}[\{1/2 - M23/2, -(M23/2),$$

$$\begin{aligned}
& \frac{1}{2} + \frac{S3}{2}, \frac{1}{2} + \frac{S3}{2}, -(\frac{1}{2}) - \frac{M23}{2} - \frac{S2}{2} - \frac{T2}{2}, -(\frac{M23}{2}) - \frac{S2}{2} - \frac{T2}{2}, \\
& \{ \frac{1}{2}, -(\frac{M23}{2}) - \frac{S2}{2}, \frac{1}{2} - \frac{M23}{2} - \frac{S2}{2}, \frac{1}{2} + \frac{S3}{2} + \frac{T3}{2}, \frac{3}{2} + \frac{S3}{2} + \frac{T3}{2} \}, 1] \\
& \text{Sec}[\frac{1}{2} \pi (S2 + T2)] \text{Sec}[\frac{1}{2} \pi (S3 + T3)] \text{Sin}[(\pi S2)/2] \\
& \text{Sin}[(\pi S3)/2] \text{Sin}[(\pi T2)/2] \text{Sin}[(\pi T3)/2] + \\
& A4[M23, S3] \times A4[1 + M23 + S2 + S3, T2] \text{HypergeometricPFQ} [\{ \frac{1}{2} + \frac{S3}{2}, \frac{1}{2} + \frac{S3}{2}, \\
& \frac{1}{2} + \frac{M23}{2} + \frac{S2}{2} + \frac{S3}{2}, \frac{3}{2} + \frac{M23}{2} + \frac{S2}{2} + \frac{S3}{2}, \frac{1}{2} - \frac{T3}{2}, -(\frac{T3}{2}) \}, \\
& \{ \frac{1}{2}, \frac{1}{2} + \frac{M23}{2} + \frac{S3}{2}, \frac{3}{2} + \frac{M23}{2} + \frac{S3}{2}, \frac{3}{2} + \frac{M23}{2} + \frac{S2}{2} + \frac{S3}{2} + \frac{T2}{2}, \\
& \frac{2}{2} + \frac{M23}{2} + \frac{S2}{2} + \frac{S3}{2} + \frac{T2}{2} \}, 1] \text{Sec}[\frac{1}{2} \pi (S2 + T2)] \text{Sec}[\frac{1}{2} \pi (S3 + T3)] \\
& \text{Sin}[(M23 \pi)/2] (2 \text{Csc}[\frac{1}{2} \pi (M23 + S2 + S3 + T2)] \text{Sin}[(\pi S3)/2]^2 + \\
& \text{Sec}[\frac{1}{2} \pi (M23 + S2 + S3 + T2)] \text{Sin}[\pi S3] \text{Sin}[\pi T2] \text{Sin}[(\pi T3)/2] - \\
& T3 A4[M23, 1 + S3] \times A4[2 + M23 + S2 + S3, T2] \text{HypergeometricPFQ} [\{ \frac{1}{2} + \frac{S3}{2}, \frac{3}{2} + \frac{S3}{2}, \\
& \frac{3}{2} + \frac{M23}{2} + \frac{S2}{2} + \frac{S3}{2}, \frac{2}{2} + \frac{M23}{2} + \frac{S2}{2} + \frac{S3}{2}, \frac{1}{2} - \frac{T3}{2}, \frac{1}{2} - \frac{T3}{2} \}, \\
& \{ \frac{3}{2}, \frac{3}{2} + \frac{M23}{2} + \frac{S3}{2}, \frac{2}{2} + \frac{M23}{2} + \frac{S3}{2}, \frac{2}{2} + \frac{M23}{2} + \frac{S2}{2} + \frac{S3}{2} + \frac{T2}{2}, \\
& \frac{5}{2} + \frac{M23}{2} + \frac{S2}{2} + \frac{S3}{2} + \frac{T2}{2} \}, 1] \text{Sec}[\frac{1}{2} \pi (S2 + T2)] \text{Sec}[\frac{1}{2} \pi (S3 + T3)] \\
& \text{Sin}[(M23 \pi)/2] (2 \text{Csc}[\frac{1}{2} \pi (M23 + S2 + S3 + T2)] \text{Sin}[(\pi S3)/2]^2 + \\
& \text{Sec}[\frac{1}{2} \pi (M23 + S2 + S3 + T2)] \text{Sin}[\pi S3] \text{Sin}[\pi T2] \text{Sin}[(\pi T3)/2] - \\
& 4 T2 A4[M23, -1 + S2 + T2] \times A4[M23 + S2 + S3 + T2, T3] \text{HypergeometricPFQ} [ \\
& \{ \frac{1}{2} - \frac{T2}{2}, \frac{1}{2} - \frac{T2}{2}, -(\frac{M23}{2}) - \frac{S2}{2} - \frac{T2}{2}, \frac{1}{2} - \frac{M23}{2} - \frac{S2}{2} - \frac{T2}{2}, \\
& -(\frac{1}{2}) - \frac{M23}{2} - \frac{S2}{2} - \frac{S3}{2} - \frac{T2}{2} - \frac{T3}{2}, -(\frac{M23}{2}) - \frac{S2}{2} - \frac{S3}{2} - \frac{T2}{2} - \frac{T3}{2} \}, \\
& \{ \frac{3}{2}, \frac{1}{2} - \frac{S2}{2} - \frac{T2}{2}, \frac{1}{2} - \frac{S2}{2} - \frac{T2}{2}, -(\frac{M23}{2}) - \frac{S2}{2} - \frac{S3}{2} - \frac{T2}{2}, \\
& \frac{1}{2} - \frac{M23}{2} - \frac{S2}{2} - \frac{S3}{2} - \frac{T2}{2} \}, 1] \\
& \text{Sec}[\frac{1}{2} \pi (M23 + S2 + T2)] \text{Sec}[\frac{1}{2} \pi (S3 + T3)] \text{Sin}[(M23 \pi)/2] \\
& \text{Sin}[(\pi S3)/2] \text{Sin}[\frac{1}{2} \pi (S2 + T2)] \text{Sin}[(\pi T3)/2] + \\
& 4 A4[M23, S2 + T2] \times A4[1 + M23 + S2 + S3 + T2, T3] \text{HypergeometricPFQ} [ \\
& \{ \frac{1}{2} - \frac{T2}{2}, -(\frac{1}{2}) - \frac{M23}{2} - \frac{S2}{2} - \frac{T2}{2}, -(\frac{M23}{2}) - \frac{S2}{2} - \frac{T2}{2}, -(\frac{T2}{2}), \\
& -1 - \frac{M23}{2} - \frac{S2}{2} - \frac{S3}{2} - \frac{T2}{2} - \frac{T3}{2}, -(\frac{1}{2}) - \frac{M23}{2} - \frac{S2}{2} - \frac{S3}{2} - \frac{T2}{2} - \frac{T3}{2} \}, \\
& \{ \frac{1}{2}, -(\frac{S2}{2}) - \frac{T2}{2}, \frac{1}{2} - \frac{S2}{2} - \frac{T2}{2}, -(\frac{1}{2}) - \frac{M23}{2} - \frac{S2}{2} - \frac{S3}{2} - \frac{T2}{2}, \\
& -(\frac{M23}{2}) - \frac{S2}{2} - \frac{S3}{2} - \frac{T2}{2} \}, 1] \text{Sec}[\frac{1}{2} \pi (M23 + S2 + T2)] \text{Sec}[\frac{1}{2} \pi (S3 + T3)] \\
& \text{Sin}[(M23 \pi)/2] \text{Sin}[(\pi S3)/2] \text{Sin}[\frac{1}{2} \pi (S2 + T2)] \text{Sin}[(\pi T3)/2] + \\
& 2 T2 A4[M23, 1 + S2] \times A4[2 + M23 + S2 + S3, T3] \text{HypergeometricPFQ} [ \\
& \{ \frac{1}{2} + \frac{S2}{2}, \frac{3}{2} + \frac{S2}{2}, \frac{3}{2} + \frac{M23}{2} + \frac{S2}{2} + \frac{S3}{2}, \frac{2}{2} + \frac{M23}{2} + \frac{S2}{2} + \frac{S3}{2}, \\
& \frac{1}{2} - \frac{T2}{2}, \frac{1}{2} - \frac{T2}{2} \}, \{ \frac{3}{2}, \frac{3}{2} + \frac{M23}{2} + \frac{S2}{2}, \frac{2}{2} + \frac{M23}{2} + \frac{S2}{2}, \\
& \frac{2}{2} + \frac{M23}{2} + \frac{S2}{2} + \frac{S3}{2} + \frac{T3}{2}, \frac{5}{2} + \frac{M23}{2} + \frac{S2}{2} + \frac{S3}{2} + \frac{T3}{2} \}, 1] \\
& \text{Sec}[\frac{1}{2} \pi (S3 + T3)] \text{Sin}[(M23 \pi)/2] (2 \text{Sec}[\frac{1}{2} \pi (M23 + S2)] \text{Sec}[\frac{1}{2} \pi (S2 + T2)] \\
& \text{Sin}[(\pi S2)/2]^2 \text{Sin}[(\pi S3)/2] \text{Sin}[(\pi T2)/2] \text{Sin}[(\pi T3)/2] - \\
& \text{Csc}[\frac{1}{2} \pi (M23 + S2)] \text{Sec}[\frac{1}{2} \pi (S2 + T2)] \text{Sin}[\pi S2] \text{Sin}[(\pi S3)/2] \text{Sin}[(\pi T2)/2] \\
& \text{Sin}[(\pi T3)/2] + \text{Csc}[\frac{1}{2} \pi (M23 + S2 + S3 + T3)] \text{Sin}[(\pi S2)/2] \text{Sin}[\pi T3] + \\
& 2 A4[M23, S2] \times A4[1 + M23 + S2 + S3, T3] \text{HypergeometricPFQ} [\{ \frac{1}{2} + \frac{S2}{2}, \\
& \frac{1}{2} + \frac{S2}{2}, \frac{1}{2} + \frac{M23}{2} + \frac{S2}{2} + \frac{S3}{2}, \frac{3}{2} + \frac{M23}{2} + \frac{S2}{2} + \frac{S3}{2}, \frac{1}{2} - \frac{T2}{2}, -(\frac{T2}{2}) \}, \\
& \{ \frac{1}{2}, \frac{1}{2} + \frac{M23}{2} + \frac{S2}{2}, \frac{3}{2} + \frac{M23}{2} + \frac{S2}{2}, \frac{3}{2} + \frac{M23}{2} + \frac{S2}{2} + \frac{S3}{2} + \frac{T3}{2}, \\
& \frac{2}{2} + \frac{M23}{2} + \frac{S2}{2} + \frac{S3}{2} + \frac{T3}{2} \}, 1] \text{Sec}[\frac{1}{2} \pi (S2 + T2)] \\
& \text{Sec}[\frac{1}{2} \pi (S3 + T3)] \text{Sin}[(M23 \pi)/2] (\text{Csc}[\frac{1}{2} \pi (M23 + S2)] \text{Sin}[\pi S2] \\
& \text{Sin}[(\pi S3)/2] \text{Sin}[(\pi T2)/2] \text{Sin}[(\pi T3)/2] - \text{Sin}[(\pi S2)/2]
\end{aligned}$$

$$\begin{aligned}
& (2 \operatorname{Sec}[1/2 \pi (M23 + S2)] \operatorname{Sin}[(\pi S2)/2] \operatorname{Sin}[(\pi S3)/2] \operatorname{Sin}[(\pi T2)/2] \operatorname{Sin}[(\pi T3)/2] + \operatorname{Cos}[1/2 \pi (S2 + T2)] \operatorname{Csc}[1/2 \pi (M23 + S2 + S3 + T3)] \operatorname{Sin}[\pi T3])) + \\
& 2 A4[M23, S3 + T3] \times A4[T2, 1 + M23 + S2 + S3 + T3] \operatorname{HypergeometricPFQ} [ \\
& \{1/2 - T3/2, -(1/2) - M23/2 - S3/2 - T3/2, -(M23/2) - S3/2 - T3/2, -1 - M23/2 - \\
& S2/2 - S3/2 - T2/2 - T3/2, -(1/2) - M23/2 - S2/2 - S3/2 - T2/2 - T3/2, -(T3/2)\}, \\
& \{1/2, -(S3/2) - T3/2, 1/2 - S3/2 - T3/2, -(1/2) - M23/2 - S2/2 - S3/2 - T3/2, \\
& -(M23/2) - S2/2 - S3/2 - T3/2\}, 1] \operatorname{Sec}[1/2 \pi (S2 + T2)] \\
& \operatorname{Sin}[(M23 \pi)/2] (2 \operatorname{Sec}[1/2 \pi (M23 + S3 + T3)] \operatorname{Sin}[(\pi S2)/2] \operatorname{Sin}[(\pi T2)/2] - \\
& \operatorname{Csc}[1/2 \pi (M23 + S2 + S3 + T2 + T3)] \operatorname{Sin}[\pi T2]) \operatorname{Sin}[1/2 \pi (S3 + T3)] + \\
& 2 T3 A4[M23, -1 + S3 + T3] \times A4[T2, M23 + S2 + S3 + T3] \operatorname{HypergeometricPFQ} [ \\
& \{1/2 - T3/2, 1 - T3/2, -(M23/2) - S3/2 - T3/2, 1/2 - M23/2 - S3/2 - T3/2, \\
& -(1/2) - M23/2 - S2/2 - S3/2 - T2/2 - T3/2, -(M23/2) - S2/2 - S3/2 - T2/2 - T3/2\}, \\
& \{3/2, 1/2 - S3/2 - T3/2, 1 - S3/2 - T3/2, -(M23/2) - S2/2 - S3/2 - T3/2, \\
& 1/2 - M23/2 - S2/2 - S3/2 - T3/2\}, 1] \operatorname{Sec}[1/2 \pi (S2 + T2)] \\
& \operatorname{Sin}[(M23 \pi)/2] (-2 \operatorname{Sec}[1/2 \pi (M23 + S3 + T3)] \operatorname{Sin}[(\pi S2)/2] \operatorname{Sin}[(\pi T2)/2] + \\
& \operatorname{Csc}[1/2 \pi (M23 + S2 + S3 + T2 + T3)] \operatorname{Sin}[\pi T2]) \operatorname{Sin}[1/2 \pi (S3 + T3)] - \\
& 4 M23 A4[-1 + M23 + S2, T2] \times A4[1 + S3, T3] \operatorname{Cos}[1/2 \pi (2 + S2)] \\
& \operatorname{Cos}[1/2 \pi (2 + S3)] \operatorname{Cos}[1/2 \pi (1 + T2)] \operatorname{Cos}[1/2 \pi (1 + T3)] \\
& \operatorname{HypergeometricPFQ} [\{1/2 - M23/2, 1 - M23/2, 1 + S3/2, \\
& 3/2 + S3/2, -(M23/2) - S2/2 - T2/2, 1/2 - M23/2 - S2/2 - T2/2\}, \\
& \{3/2, 1/2 - M23/2 - S2/2, 1 - M23/2 - S2/2, 3/2 + S3/2 + T3/2, 2 + S3/2 + T3/2\}, 1] \\
& \operatorname{Sec}[1/2 \pi (3 + S2 + T2)] \operatorname{Sec}[1/2 \pi (3 + S3 + T3)] \operatorname{Tan}[(\pi S2)/2] \\
& \operatorname{Tan}[(\pi S3)/2] \operatorname{Tan}[1/2 \pi (S2 + T2)] \operatorname{Tan}[1/2 \pi (S3 + T3)];
\end{aligned}$$

Full (120-permutation symmetric) 5 - point Veneziano amplitude in terms of 4-point amplitudes and 3F2 hypergeometric functions.

```

A5InTermsOf3F2 [S2_, T2_, S3_, T3_, M23_] :=
A4[S2, T2] * A4[T3, M23 + S3] HypergeometricPFQ [{-M23, 1 + S2, -1 - M23 - S3 - T3},
{-M23 - S3, 2 + S2 + T2}, 1] + A4[S2, T2] * A4[T3, -2 - M23 - S3 - T3]
HypergeometricPFQ [{-M23, 1 + S2, -1 - M23 - S3 - T3}, {-M23 - S3, 2 + S2 + T2}, 1] +
A4[-2 - M23 - S2 - T2, S2] * A4[T3, -2 - M23 - S3 - T3]
HypergeometricPFQ [{-M23, 1 + S2, 1 + T3}, {-M23 - S3, -M23 - T2}, 1] +
A4[S3, T3] * A4[T2, -2 - M23 - S2 - T2] HypergeometricPFQ [
{-M23, 1 + S3, -1 - M23 - S2 - T2}, {-M23 - S2, 2 + S3 + T3}, 1] +
A4[-2 - M23 - S2 - T2, T2] * A4[T3, -2 - S3 - T3] HypergeometricPFQ [
{-M23, 1 + S3, -1 - M23 - S2 - T2}, {-M23 - S2, 2 + S3 + T3}, 1] +
A4[T2, -2 - M23 - S2 - T2] * A4[-2 - M23 - S3 - T3, S3]
HypergeometricPFQ [{-M23, 1 + S3, 1 + T2}, {-M23 - S2, -M23 - T3}, 1] +
A4[S3, -2 - S3 - T3] * A4[-2 - M23 - S2 - T2, S2]
HypergeometricPFQ [{-M23, -1 - M23 - S2 - T2, 1 + T3}, {-M23 - T2, 2 + S3 + T3}, 1] +
A4[S2, -2 - M23 - S2 - T2] * A4[T3, S3] HypergeometricPFQ [{-M23, -1 - M23 - S2 - T2,
1 + T3}, {-M23 - T2, 2 + S3 + T3}, 1] + A4[S3, -2 - M23 - S3 - T3] * A4[T2, S2]
HypergeometricPFQ [{-M23, 1 + T2, -1 - M23 - S3 - T3}, {2 + S2 + T2, -M23 - T3}, 1] -
2 A4[S3, M23] * A4[T2, 1 + M23 + S2 + S3] Cos[1/2 (-1 - M23)  $\pi$ ] Csc[ $\pi$  (1 + M23 + S3)]
HypergeometricPFQ [{1 + S3, 2 + M23 + S2 + S3, -T3}, {2 + M23 + S3, 3 + M23 + S2 + S3 + T2},
1] Sin[1/2 (-1 - M23)  $\pi$  -  $\pi$  S3] - 2 A4[S2, -3 - M23 - S2 - S3 - T2 - T3] *
A4[-2 - M23 - S3 - T3, M23] Cos[1/2 (-1 - M23)  $\pi$ ] Csc[ $\pi$  (-1 - S3 - T3)]
HypergeometricPFQ [{-S3, -1 - M23 - S3 - T3, -2 - M23 - S2 - S3 - T2 - T3},
{-S3 - T3, -1 - M23 - S3 - T2 - T3}, 1] Sin[1/2 (-1 - M23)  $\pi$  -  $\pi$  (-2 - M23 - S3 - T3)] -
2 A4[T2, -3 - M23 - S2 - S3 - T2 - T3] * A4[-2 - M23 - S3 - T3, M23]
Cos[1/2 (-1 - M23)  $\pi$ ] Csc[ $\pi$  (-1 - S3 - T3)]
HypergeometricPFQ [{-1 - M23 - S3 - T3, -2 - M23 - S2 - S3 - T2 - T3, -T3},
{-S3 - T3, -1 - M23 - S2 - S3 - T3}, 1] Sin[1/2 (-1 - M23)  $\pi$  -  $\pi$  (-2 - M23 - S3 - T3)];

```

Full (120-permutation symmetric) 5 - point Veneziano amplitude in terms of 4-point amplitudes and 3F2 hypergeometric functions, an alternate presentation

```

A5InTermsOf3F2AlternateExpression [S2_, T2_, S3_, T3_, M23_] :=
A4[S2, T2] * A4[T3, M23 + S3] HypergeometricPFQ [{-M23, 1 + S2, -1 - M23 - S3 - T3},
{-M23 - S3, 2 + S2 + T2}, 1] + A4[S2, T2] * A4[T3, -2 - M23 - S3 - T3]
HypergeometricPFQ [{-M23, 1 + S2, -1 - M23 - S3 - T3}, {-M23 - S3, 2 + S2 + T2}, 1] +
A4[S3, T3] * A4[T2, -2 - M23 - S2 - T2]
HypergeometricPFQ [{-M23, 1 + S3, -1 - M23 - S2 - T2}, {-M23 - S2, 2 + S3 + T3}, 1] +
A4[-2 - M23 - S2 - T2, T2] * A4[T3, -2 - S3 - T3]
HypergeometricPFQ [{-M23, 1 + S3, -1 - M23 - S2 - T2}, {-M23 - S2, 2 + S3 + T3}, 1] +
A4[S3, -2 - S3 - T3] * A4[-2 - M23 - S2 - T2, S2]
HypergeometricPFQ [{-M23, -1 - M23 - S2 - T2, 1 + T3}, {-M23 - T2, 2 + S3 + T3}, 1] +

```

$$\begin{aligned}
& A4[S2, -2 - M23 - S2 - T2] \times A4[T3, S3] \\
& \quad \text{HypergeometricPFQ} \left[ \{-M23, -1 - M23 - S2 - T2, 1 + T3\}, \{-M23 - T2, 2 + S3 + T3\}, 1 \right] + \\
& A4[S3, -2 - M23 - S3 - T3] \times A4[T2, S2] \\
& \quad \text{HypergeometricPFQ} \left[ \{-M23, 1 + T2, -1 - M23 - S3 - T3\}, \{2 + S2 + T2, -M23 - T3\}, 1 \right] - \\
& 2 A4[S3, M23] \times A4[T2, 1 + M23 + S2 + S3] \cos\left[\frac{1}{2}(-1 - M23)\pi\right] \\
& \quad \csc[\pi(1 + M23 + S3)] \text{HypergeometricPFQ} \left[ \{1 + S3, 2 + M23 + S2 + S3, -T3\}, \right. \\
& \quad \left. \{2 + M23 + S3, 3 + M23 + S2 + S3 + T2\}, 1 \right] \sin\left[\frac{1}{2}(-1 - M23)\pi - \pi S3\right] - \\
& (2 A4[M23, S3 + T3] \times A4[T2, 1 + M23 + S2 + S3 + T3] \text{HypergeometricPFQ} \left[ \{-1 - M23 - S3 - T3, \right. \\
& \quad \left. -2 - M23 - S2 - S3 - T2 - T3, -T3\}, \{-S3 - T3, -1 - M23 - S2 - S3 - T3\}, 1 \right] \\
& \quad \sin[(-1 - M23)\pi] \sin[\pi T2]) / (\cos[\pi(S2 + T2)] - \cos[\pi(S2 + T2 + 2(1 + M23 + S3 + T3))]) - \\
& A4[S3, T3] \times A4[T2, M23 + S2] \csc[\pi(1 + M23 + S2 + T2)] \csc[\pi(S3 + T3)] \\
& \quad \text{HypergeometricPFQ} \left[ \{-M23, 1 + S3, -1 - M23 - S2 - T2\}, \{-M23 - S2, 2 + S3 + T3\}, 1 \right] \\
& \quad \sin[\pi S3] \sin[\pi T2] - 2 A4[S3, M23] \times A4[1 + M23 + S2 + S3, T2] \cos\left[\frac{1}{2}(-1 - M23)\pi\right] \\
& \quad \csc[\pi(S2 + T2)] \text{HypergeometricPFQ} \left[ \{1 + S3, 2 + M23 + S2 + S3, -T3\}, \right. \\
& \quad \left. \{2 + M23 + S3, 3 + M23 + S2 + S3 + T2\}, 1 \right] \sin\left[\frac{1}{2}(-1 - M23)\pi\right] \\
& \quad (\csc[\pi(1 + M23 + S3)] \sin[\pi S2] + \csc[\pi(1 + M23 + S2 + S3 + T2)] \sin[\pi T2]) - \\
& 2 A4[S2, -3 - M23 - S2 - S3 - T2 - T3] \times A4[-2 - M23 - S3 - T3, M23] \\
& \quad \cos\left[\frac{1}{2}(-1 - M23)\pi\right] \csc[\pi(-1 - S3 - T3)] \\
& \quad \text{HypergeometricPFQ} \left[ \{-S3, -1 - M23 - S3 - T3, -2 - M23 - S2 - S3 - T2 - T3\}, \right. \\
& \quad \left. \{-S3 - T3, -1 - M23 - S3 - T2 - T3\}, 1 \right] \sin\left[\frac{1}{2}(-1 - M23)\pi - \pi(-2 - M23 - S3 - T3)\right] - \\
& 2 A4[T2, -3 - M23 - S2 - S3 - T2 - T3] \times A4[-2 - M23 - S3 - T3, M23] \\
& \quad \cos\left[\frac{1}{2}(-1 - M23)\pi\right] \csc[\pi(-1 - S3 - T3)] \\
& \quad \text{HypergeometricPFQ} \left[ \{-1 - M23 - S3 - T3, -2 - M23 - S2 - S3 - T2 - T3, -T3\}, \right. \\
& \quad \left. \{-S3 - T3, -1 - M23 - S2 - S3 - T3\}, 1 \right] \sin\left[\frac{1}{2}(-1 - M23)\pi - \pi(-2 - M23 - S3 - T3)\right] - \\
& (2 A4[M23, S2 + T2] \times A4[T3, 1 + M23 + S2 + S3 + T2] \text{HypergeometricPFQ} \left[ \{-1 - M23 - S2 - T2, \right. \\
& \quad \left. -T2, -2 - M23 - S2 - S3 - T2 - T3\}, \{-S2 - T2, -1 - M23 - S2 - S3 - T2\}, 1 \right] \\
& \quad \sin[(-1 - M23)\pi] \sin[\pi T3]) / (\cos[\pi(S3 + T3)] - \cos[\pi(S3 + 2(1 + M23 + S2 + T2) + T3)]) - \\
& A4[S2, T2] \times A4[T3, M23 + S3] \csc[\pi(S2 + T2)] \csc[\pi(1 + M23 + S3 + T3)] \\
& \quad \text{HypergeometricPFQ} \left[ \{-M23, 1 + S2, -1 - M23 - S3 - T3\}, \{-M23 - S3, 2 + S2 + T2\}, 1 \right] \\
& \quad \sin[\pi S2] \sin[\pi T3] - 2 A4[S2, M23] \times A4[1 + M23 + S2 + S3, T3] \cos\left[\frac{1}{2}(-1 - M23)\pi\right] \\
& \quad \csc[\pi(S3 + T3)] \text{HypergeometricPFQ} \left[ \{1 + S2, 2 + M23 + S2 + S3, -T2\}, \right. \\
& \quad \left. \{2 + M23 + S2, 3 + M23 + S2 + S3 + T3\}, 1 \right] \sin\left[\frac{1}{2}(-1 - M23)\pi\right] \\
& \quad (\csc[\pi(1 + M23 + S2)] \sin[\pi S3] + \csc[\pi(1 + M23 + S2 + S3 + T3)] \sin[\pi T3])
\end{aligned}$$
